# Supplementary material for: ABC of Order Dependencies
Source: arXiv:1905.11948 source file (2020-02-28)
Supplement: Supplementary file 1 [file appendix.tex]

%\section{Proofs}\label{sec:proofs}

\subsection{Theorem~\ref{them:best}}

\proof{
Consider the case of IBs in a prefix $T\mbox{[}i-1\mbox{]}$. Tuple $s_{k, i-1}$ is the smallest maximal tuple of ${\sf IB}_{k, i-1}$. Since 
%$s_{k-1, i-1} \preceq_{\Delta t, \overline{\textbf{Y}}} t_i$
$d \mbox{(} s_{k-1, i-1}.\textbf{Y}, t_i.\textbf{Y}  \mbox{)}$ $\geq - \Delta$, a tuple $t_i$ is the maximal tuple of a monotonic band ${\sf IB}_{k-1, i-1} \cup t_i$ with length $k$. In addition, $d\mbox{(}t_i.\textbf{Y}, s_{k-1, i-1}.\textbf{Y}\mbox{)} \geq 0$, therefore, $t_i$ is the smallest maximal tuple among IBs with length $k$ in a prefix $T\mbox{[}i\mbox{]}$.

Accordingly, consider the case of DBs in a prefix $T\mbox{[}i-1\mbox{]}$. A tuple $l_{k, i-1}$ is the largest minimal tuple of ${\sf DB}_{k, i-1}$. As 
%$l_{k-1, i-1} \preceq_{\Delta t, \overline{\textbf{Y}}} t_i$
$d \mbox{(} l_{k-1, i-1}.\textbf{Y}, t_i.\textbf{Y}  \mbox{)}$ $\leq \Delta$, a tuple $t_i$ is the minimal tuple of a monotonic band ${\sf DB}_{k-1, i-1} \cup t_i$ with the length $k$. In addition, $d\mbox{(}t_i, l_{k-1, i-1}\mbox{)} \leq 0$, thus, $t_i$ is a largest minimal tuple among DBs with length $k$ in prefix $T\mbox{[}i\mbox{]}$.
}

\subsection{Theorem~\ref{lemma:lmb}}
\proof{
To find LMBs in the sequence of tuples $T$, the key is to find the length of a LMB by identifying the best tuples in $T$. Since a tuple $B_{\sf inc}\mbox{[}k_1\mbox{]}$ is updated by the algorithm by $\max\mbox{(}s_{k_1-1}.\textbf{Y}, t_i.\textbf{Y}\mbox{)}$, where $d\mbox{(}t_i.\textbf{Y}, s_{k_1-1}.\textbf{Y}\mbox{)} > 0$, the corresponding band $\sf{IB}_{k_1, i}$ is a IB with smallest maximal tuples that ends at tuple $t_i$ in the sequence $T\mbox{[}i\mbox{]}$. It is also a monotonic band with the shortest length, as $k_1$ is the smallest index in $B_{\sf inc}$. Similarly, $\sf{IB}_{k_2, i}$ is a {\sf IB} of the longest length among IBs with the smallest maximal tuple that ends at $t_i$ in the sequence $T\mbox{[}i\mbox{]}$. 

For each $t_i \in T$, we know that the lengths of IBs with
the smallest maximal tuples that ends at $t_i$ fall into the range
$\mbox{[}k_1, k_2\mbox{]}$. The length of a LIB in $T\mbox{[}i\mbox{]}$ is the maximal value in array $P_{\sf inc}\mbox{[}i\mbox{]}$. Accordingly, Algorithm~\ref{alg:lmb} finds a ${\sf LDB}$ with the largest minimal tuple in the sequence $T$.

For each tuple $t_i$ in the sequence $T$ of length $n$, it takes time $O\mbox{(}\log n\mbox{)}$  to update array $B_{\sf inc}$, $B_{\sf dec}$, $P_{\sf inc}$ and $P_{\sf dec}$. Therefore, it takes time $O\mbox{(}n\log n\mbox{)}$ to find a $\sf LMB$ in the sequence $T$. Each tuple $t_i$ inserts maximally $\Delta + 1$ values into arrays $P_{\sf inc}$ and $P_{\sf dec}$; thus, Algorithm~\ref{alg:lmb} takes space $O\mbox{((}\Delta + 1\mbox{)}n\mbox{)}$.
}

\subsection{Lemma~\ref{lemma:piece}}
\proof{
While processing each tuple $t_i$ in the sequence of tuples $T$ of length $n$ two maps $M_{\sf inc}$ and $M_{\sf dec}$ are updated by the algorithm up to $(\Delta +1)$ times, respectively. Therefore, Algorithm~\ref{alg:piece} takes time $O\mbox{(}\Delta + 1\mbox{)} \cdot n$. 
}

\subsection{Theorem~\ref{theo:series}}
\proof{
Algorithm~\ref{alg:series} applies dynamic programming to solve Equation~\ref{eq:opt}. 
The recurrence in Equation~\ref{eq:opt} specifies that the series in
a prefix $T\mbox{[}i\mbox{]}$ are selected among $i$ alternative options: (1) a
singleton series consisting of $t_i$, and the series in a prefix
$T\mbox{[}i-1\mbox{]}$; (2) a series of length $2$ consisting of $\{ t_i, t_{i-1} \}$, and the series in a prefix $T\mbox{[}i-2\mbox{]}$, etc.; and finally, a series of length $i$ consisting of all tuples in a prefix $T\mbox{[}i\mbox{]}$. Therefore, it requires $O\mbox{(}n\mbox{)}$ iterations to find series in a prefix $T\mbox{[}j\mbox{]}$, where each iteration takes time $O\mbox{(}n\log n\mbox{)}$, according to Lemma~\ref{lemma:lmb}. There are in total $n$ tuples in the sequence $T$, thus, Algorithm~\ref{alg:series} takes time $O\mbox{(}n^3\log n\mbox{)}$.
}

\subsection{Theorem~\ref{theo:greedy}}
\proof{
The proposed piece-based abcOD discovery algorithm first finds all pieces in the sequence $T$ of length $n$, which takes time $O\mbox{(}\Delta t + 1\mbox{)}\cdot n$. Assume the number of pieces is $m$, the algorithm applies dynamic programming on $m$ pieces, similarly as Algorithm~\ref{alg:series}, which takes time $O\mbox{(}m^2n\log n\mbox{)}$. Therefore, the overall time complexity is $O\mbox{(}m^2n\log n\mbox{)}$.
}

\subsection{Theorem~\ref{theo2:greedy}}
\proof{
Consider the discovery of unidirectional abcODs case, where without loss of generality all series are increasing; that is, the LMBs in each series are LIBs. We show that the pieces-based  algorithm finds the optimal solution in the prefix $T\mbox{[}i\mbox{]}$, which ends at the piece $P_i=\{t_{i-m+1}, \cdots, t_i\}$ of length $m$.

The last tuple $t_i$ in the prefix $T\mbox{[}i\mbox{]}$ cannot be an outlier of a series in the optimal solution of $T\mbox{[}i\mbox{]}$; otherwise, the profit of solution, where $t_i$ is a singleton series, is always larger, i.e., ${\sf OPT}\mbox{(}i\mbox{)} < {\sf OPT}\mbox{(}i-1\mbox{)} + 1$ according to Equation~\ref{eq:opt}. On the other hand, as every tuple in a piece $P_i=\{t_{i-m+1}, \cdots, t_i\}$ belongs to the same sets of pre-pieces, there is no outliers that violates LIB in $P_i$; that is, $g\mbox{(}T\mbox{[}i-m+1, i]\mbox{)} = m^2$ and $g\mbox{(}T\mbox{[}i-k+1, i\mbox{]}\mbox{)} = k^2$.

Assume that the piece-based discovery algorithm does not find the optimal solution in $T\mbox{[}i\mbox{]}$; i.e., there exists tuple $t_{i-k} \in P_i, 0 \leq k \leq m-1$ in the optimal solution that splits $P_i$ into two series: $\{t_{i-m+1}, \cdots, t_{i-k}\}$ and $\{t_{i-k+1}, \cdots, t_i\}$, where the profit is ${\sf OPT}\mbox{(}i-k\mbox{)} + k^2$. We next prove that this assumption does not hold, i.e., ${\sf OPT}\mbox{(}i\mbox{)} - {\sf OPT}\mbox{(}i-k\mbox{)} \geq k^2 $. 

Consider that a tuple $t_{i-j+1}$ is the first tuple in the last series $S_{i-m}$ of the optimal solution ${\sf OPT}\mbox{(}i-m\mbox{)}$, where the length of a LIBs in series $S_{i-m}$ is $l$, i.e., $j \geq m + 1, l >0$; and the maximal number of consecutive outliers in $T\mbox{[}i-m\mbox{]}$ is $q$. According to Theorem~\ref{them:best}, $\{t_{i-m+1}, \cdots, t_{i}\}$ extends the length of LIB in $S_{i-m}$ by $m-k$ without increasing $q$. That is
\[
{\sf OPT}\mbox{(}i\mbox{)} = {\sf OPT}\mbox{(}i-j\mbox{)} + \mbox{(}l+m\mbox{)}^2
\]
Similarly, 
\[
{\sf OPT}\mbox{(}i-k\mbox{)} = {\sf OPT}\mbox{(}i-j\mbox{)} + \mbox{(}l+m-k\mbox{)}^2
\]
Which means,
\[
{\sf OPT}\mbox{(}i\mbox{)} - {\sf OPT}\mbox{(}i-k\mbox{)} = \mbox{(}l+m\mbox{)}^2 - \mbox{(}l+m-k\mbox{)}^2 = 2k\mbox{(}l+m\mbox{)} > k^2
\]

Thus, the proposed piece-based algorithm finds the optimal solution in the sequence $T$, where LMBs in all series are increasing. Accordingly, the proposed piece-based algorithm finds the optimal solution in the sequence $T$, where LMB in all series are decreasing. 
}

%\section{Optimal vs Greedy Algorithm}\label{app:lmb}

%Based on Theorem~\ref{theo2:greedy}, the {\sc LMB} algorithm finds the optimal solution over unidirectional CABODs over data where series are all increasing or all decreasing (as the \emph{Car} dataset). 
